# Supplementary material for: Current-Modulated Magnetoplasmonic Devices
Source: arXiv:1805.03926 source file (2018-05-10)
Supplement: Supplementary file 1 [file Supplementary_Information_for_Eleclectrically_Actuated_Magnetoplasmonic_Devices.pdf]

# Supplementary Information for Current-Modulated Magnetoplasmonic Devices

Mark E. Nowakowski

## Supplementary section S1: Plasmonic interferometer geometry

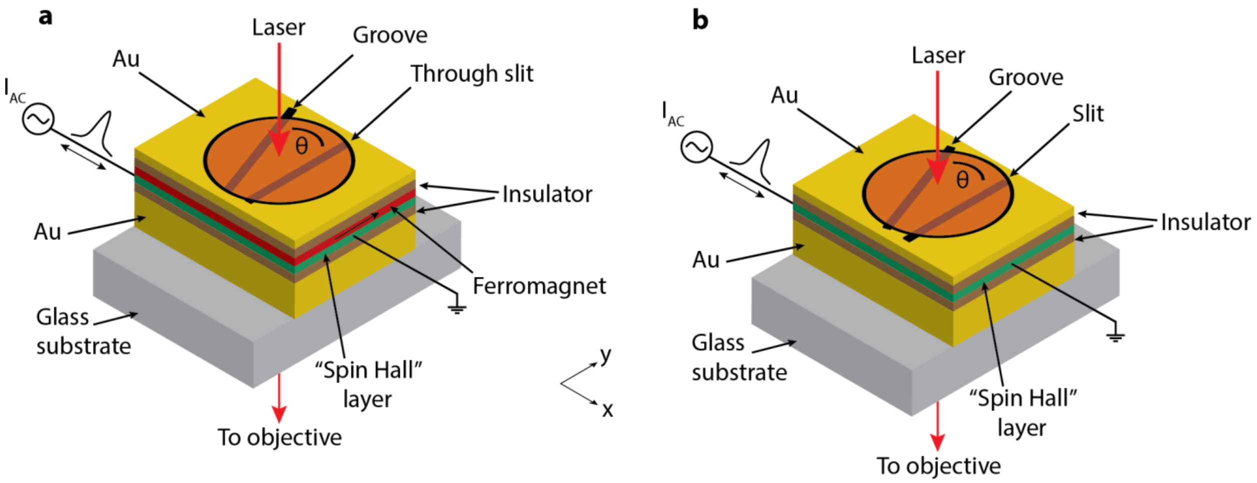


Figure S1. Schematic for plasmonic interferometer geometry for magnetoplamsonic heterostructures a) with and b) without a ferromagnetic layer

To create a plasmonic interferometer similar to ref. S1, focused ion beam (FIB) cuts are required to create a transparent slit through the stack oriented along $\hat{y}$, parallel to the magnetization direction, and a groove slanted at an angle, $\theta$, with respect to $\hat{y}$ consisting of only the capping metal. In this geometry, plasmonic light, excited by a laser source with wavelength $\lambda$, propagates along the surface and interferes with the light transmitted through the slit.

Ref. S1: V. V. Temnov et. al. Nat. Photon. **4**, 107 (2010).

## Supplementary section S2: Model with a ferromagnet

A laser of wavelength $\lambda$ excites surface plasmon polaritons (SPPs) at the surface of a heterostructure stack with the following material regions and dielectric constants:

1 (Air, $\epsilon_{air}$): $z > 0$
2 (Plasmonic metal, $\epsilon_m$): $0 > z > -a$
3 (Isolating dielectric, $\epsilon_{iso}$): $-a > z > -(a+b)$
4 (Magnet, $\epsilon_{mag}$): $-(a+b) > z > -(a+b+c)$
5 (Metal with large SOC/TI, $\epsilon_{sh}$): $-(a+b+c) > z > -(a+b+c+d)$
6 (Isolating dielectric, $\epsilon_{iso}$): $-(a+b+c+d) > z > -(a+2b+c+d)$
7 (Plasmonic metal, $\epsilon_m$): $z < -(a+2b+c+d)$

The SPP magnetic field components in each region are assumed to have the following form:

$$H_{y1} = Ae^{-k_{air}z}e^{i(k_x x-\omega t)}$$
$$H_{y2} = \left(Be^{k_m z} + Ce^{-k_m(z+a)}\right)e^{i(k_x x-\omega t)}$$

$$H_{y3} = \left(De^{k_{iso}(z+a)} + Ee^{-k_{iso}(z+(a+b))}\right)e^{i(k_x x-\omega t)}$$
$$H_{y4} = \left(Fe^{k_{mag}(z+(a+b))} + Ge^{-k_{mag}\left(z+((a+b+c))\right)}\right)e^{i(k_x x-\omega t)}$$
$$H_{y5} = \left(He^{k_{sh}\left(z+((a+b+c))\right)} + Ie^{-k_{sh}(z+(a+b+c+d))}\right)e^{i(k_x x-\omega t)}$$
$$H_{y6} = \left(Je^{k_{iso}\left(z+((a+b+c+d))\right)} + Ke^{-k_{iso}(z+(a+2b+c+d))}\right)e^{i(k_x x-\omega t)}$$
$$H_{y7} = Le^{k_m\left(z+((a+2b+c+d))\right)}e^{i(k_x x-\omega t)}$$

Maxwell Equations are used to derive the SPP electric field components
$$-\partial_z H_y = \frac{\partial D_x}{\partial t}$$
$$\partial_x H_y = \frac{\partial D_z}{\partial t}$$

The displacement field which accounts for the dielectric tensor $\epsilon$ in each material is
$$\vec{D} = \epsilon\vec{E}$$

For non-magnetic layers:
$\epsilon = \begin{pmatrix} \epsilon_{xx} & 0 & 0 \\ 0 & \epsilon_{xx} & 0 \\ 0 & 0 & \epsilon_{xx} \end{pmatrix}$, where $\epsilon_{xx}$ is the bulk dielectric value for any individual layer (i.e. $\epsilon_m$, $\epsilon_{iso}$, etc.)

For magnetic layers:
$\epsilon = \begin{pmatrix} \epsilon_{xx} & 0 & \pm\epsilon_{xz} \\ 0 & \epsilon_{xx} & 0 \\ \mp\epsilon_{xz} & 0 & \epsilon_{xx} \end{pmatrix}$, where $\epsilon_{xx}$ = $\epsilon_{mag}$ and $\epsilon_{xz}$ is an off-diagonal component generated from the magnetic polarization ($M = \pm 1$).

Calculating $\vec{D}$ generally for each layer gives
$\vec{D} = \epsilon\vec{E} = \begin{pmatrix} \epsilon_{xx} & 0 & \pm\epsilon_{xz} \\ 0 & \epsilon_{xx} & 0 \\ \mp\epsilon_{xz} & 0 & \epsilon_{xx} \end{pmatrix}\begin{pmatrix} E_x \\ E_y \\ E_z \end{pmatrix} = \begin{pmatrix} \epsilon_{xx}E_x \pm \epsilon_{xz}E_z \\ 0 \\ \epsilon_{xx}E_z \mp \epsilon_{xz}E_x \end{pmatrix}$, where $\epsilon_{xz} \to 0$ for non-magnetic layers.

Plugging into Maxwell equations gives
$$-\partial_z H_y = \frac{\partial D_x}{\partial t} = \frac{\partial}{\partial t}(\epsilon_{xx}E_x \pm \epsilon_{xz}E_z)$$
$$\partial_x H_y = \frac{\partial D_z}{\partial t} = \frac{\partial}{\partial t}(\epsilon_{xx}E_z \mp \epsilon_{xz}E_x)$$

And solving this system of equations for $E_x$ gives
$$\frac{\partial}{\partial t}E_x = \frac{\mp\left(\frac{\epsilon_{xz}}{\epsilon_{xx}}\right)\partial_x H_y - \partial_z H_y}{\left(\epsilon_{xx} + \frac{{\epsilon_{xz}}^2}{\epsilon_{xx}}\right)}$$

Assuming $E_x$ has a form similar to $H_y$, SPP electric field components in each region, *i*, are given by
$$\frac{\partial}{\partial t}E_x = -i\omega E_x$$

$$E_{xi} = \frac{\mp\left(\frac{\epsilon_{xzi}}{\epsilon_{xxi}}\right)\partial_x H_{yi} - \partial_z H_{yi}}{-i\omega\left(\epsilon_{xxi} + \frac{{\epsilon_{xzi}}^2}{\epsilon_{xxi}}\right)}$$

Taking $\epsilon_{xz}$ to first order (${\epsilon_{xz}}^2 \to 0$) gives

$$E_{xi} = \frac{\mp\left(\frac{\epsilon_{xzi}}{\epsilon_{xxi}}\right)\partial_x H_{yi} - \partial_z H_{yi}}{-i\omega\epsilon_{xxi}}$$

Next, we apply boundary conditions at each interface

$H_i = H_{i+1}$
$E_i = E_{i+1}$

In the SPP electric field equations for magnetic layer, $\frac{i\epsilon_{xz}}{\epsilon_{mag}} \to q$

The resulting boundary condition equations form a system of equations $A_{mat}X = 0$, where $A_{mat}X$ is

$$\begin{pmatrix}
1 & -1 & -e^{-k_m a} & 0 & 0 & 0 & 0 & 0 & 0 & 0 & 0 & 0 \\
\frac{k_{air}}{\epsilon_{air}} & \frac{k_m}{\epsilon_m} & -\frac{k_m}{\epsilon_m}e^{-k_m a} & 0 & 0 & 0 & 0 & 0 & 0 & 0 & 0 & 0 \\
0 & e^{-k_m a} & 1 & -1 & -e^{-k_{iso} b} & 0 & 0 & 0 & 0 & 0 & 0 & 0 \\
0 & \frac{k_m}{\epsilon_m}e^{-k_m a} & -\frac{k_m}{\epsilon_m} & -\frac{k_{iso}}{\epsilon_{iso}} & \frac{k_{iso}}{\epsilon_{iso}}e^{-k_{iso} b} & 0 & 0 & 0 & 0 & 0 & 0 & 0 \\
0 & 0 & 0 & e^{-k_{iso} b} & 1 & -1 & -e^{-k_{mag} c} & 0 & 0 & 0 & 0 & 0 \\
0 & 0 & 0 & \frac{k_{iso}}{\epsilon_{iso}}e^{-k_{iso} b} & -\frac{k_{iso}}{\epsilon_{iso}} & -\frac{(k_{mag} \pm q k_x)}{\epsilon_{mag}} & \frac{(k_{mag} \mp q k_x)}{\epsilon_{mag}}e^{-k_{mag} c} & 0 & 0 & 0 & 0 & 0 \\
0 & 0 & 0 & 0 & 0 & e^{-k_{mag} c} & 1 & -1 & -e^{-k_{sh} d} & 0 & 0 & 0 \\
0 & 0 & 0 & 0 & 0 & \frac{(k_{mag} \pm q k_x)}{\epsilon_{mag}}e^{-k_{mag} c} & -\frac{(k_{mag} \mp q k_x)}{\epsilon_{mag}} & -\frac{k_{sh}}{\epsilon_{sh}} & \frac{k_{sh}}{\epsilon_{sh}}e^{-k_{sh} d} & 0 & 0 & 0 \\
0 & 0 & 0 & 0 & 0 & 0 & 0 & e^{-k_{sh} d} & 1 & -1 & -e^{-k_{iso} b} & 0 \\
0 & 0 & 0 & 0 & 0 & 0 & 0 & \frac{k_{sh}}{\epsilon_{sh}}e^{-k_{sh} d} & -\frac{k_{sh}}{\epsilon_{sh}} & -\frac{k_{iso}}{\epsilon_{iso}} & \frac{k_{iso}}{\epsilon_{iso}}e^{-k_{iso} b} & 0 \\
0 & 0 & 0 & 0 & 0 & 0 & 0 & 0 & 0 & e^{-k_{iso} b} & 1 & -1 \\
0 & 0 & 0 & 0 & 0 & 0 & 0 & 0 & 0 & \frac{k_{iso}}{\epsilon_{iso}}e^{-k_{iso} b} & -\frac{k_{iso}}{\epsilon_{iso}} & -\frac{k_m}{\epsilon_m}
\end{pmatrix}
\begin{pmatrix} A \\ B \\ C \\ D \\ E \\ F \\ G \\ H \\ I \\ J \\ K \\ L \end{pmatrix}$$

To extract the propagation constants we must solve a system of equations that accounts for the wave equation in each heterostructure layer and enforces the boundary conditions. Note, we take $\epsilon_{xz}$ to first order in the magnetic layer again, ${\epsilon_{xz}}^2 \to 0$.

${k_x}^2 = {k_{air}}^2 + \epsilon_{air}{k_0}^2$
${k_x}^2 = {k_m}^2 + \epsilon_m{k_0}^2$
${k_x}^2 = {k_{iso}}^2 + \epsilon_{iso}{k_0}^2$
${k_x}^2 = {k_{mag}}^2 + \epsilon_{mag}{k_0}^2$
${k_x}^2 = {k_{sh}}^2 + \epsilon_{sh}{k_0}^2$
$Det[A_{mat}] = 0$

Where $k_x$ is the heterostructure propagation constant, $k_{air}$, $k_m$, $k_{iso}$, $k_{mag}$, and $k_{sh}$ are the perpendicular wave vector components in each region, and $k_0 = \frac{\omega}{c} = \frac{2\pi}{\lambda}$. This system is then solved numerically. The magnetoplasmonic signal is obtained after solving this system for both magnetic polarization conditions ($M = \pm 1$).

$$\left|\Delta k_{mp}\right| = |k_x^{M=1} - k_x^{M=-1}|$$

$$L_{SPP} = \frac{1}{2Im(k_x)}$$

**Supplementary section S3: Model without a ferromagnet**

A laser of wavelength $\lambda$ excites surface plasmon polaritons (SPPs) at the surface of a heterostructure stack with the following material regions and dielectric constants:

1 (Air, $\epsilon_{air}$): $z > 0$
2 (Plasmonic metal, $\epsilon_m$): $0 > z > -a$
3 (Isolating dielectric, $\epsilon_{iso}$): $-a > z > -(a+b)$
4 (Metal with large SOC/TI, $\epsilon_{sh}$, $M = \pm 1$): $-(a+b) > z > -(a+b+l_s)$
5 (Metal with large SOC/TI, $\epsilon_{sh}$, $M = 0$): $-(a+b+l_s) > z > -(a+b+d-l_s)$
6 (Metal with large SOC/TI, $\epsilon_{sh}$, $M = \mp 1$): $-(a+b+d-l_s) > z > -(a+b+d)$
7 (Isolating dielectric, $\epsilon_{iso}$): $-(a+b+d) > z > -(a+2b+d)$
8 (Plasmonic metal, $\epsilon_m$): $z < -(a+2b+d)$

An alternating current $i_{ac}$ is assumed through the isolated metal region which generates alternating opposing spin polarizations $M = \pm 1$ in regions 4 and 6. The depth of these polarized regions within the isolated metal is determined by the material-dependent spin diffusion length $l_s$.

The SPP magnetic field components in each region are assumed to have the following form:

$$H_{y1} = Ae^{-k_{air}z}e^{i(k_x x - \omega t)}$$
$$H_{y2} = \left(Be^{k_m z} + Ce^{-k_m(z+a)}\right)e^{i(k_x x - \omega t)}$$
$$H_{y3} = \left(De^{k_{iso}(z+a)} + Ee^{-k_{iso}(z+(a+b))}\right)e^{i(k_x x - \omega t)}$$
$$H_{y4} = \left(Fe^{k_{sh}(z+(a+b))} + Ge^{-k_{sh}\left(z+((a+b+l_s))\right)}\right)e^{i(k_x x - \omega t)}$$
$$H_{y5} = \left(He^{k_{sh}\left(z+((a+b+l_s))\right)} + Ie^{-k_{sh}(z+(a+b+d-l_s))}\right)e^{i(k_x x - \omega t)}$$
$$H_{y6} = \left(Je^{k_{sh}\left(z+((a+b+d-l_s))\right)} + Ke^{-k_{sh}(z+(a+b+d))}\right)e^{i(k_x x - \omega t)}$$
$$H_{y7} = \left(Le^{k_{iso}\left(z+((a+b+d))\right)} + Me^{-k_{iso}(z+(a+2b+d))}\right)e^{i(k_x x - \omega t)}$$
$$H_{y8} = Ne^{k_m\left(z+((a+2b+d))\right)}e^{i(k_x x - \omega t)}$$

The SPP electric field components in each region are calculated in an identical manner as the previous device, taking $\epsilon_{xz}$ to first order ($\epsilon_{xz}{}^2 \to 0$) gives

$$E_{xi} = \frac{\mp\left(\frac{\epsilon_{xzi}}{\epsilon_{xxi}}\right)\partial_x H_{yi} - \partial_z H_{yi}}{-i\omega\epsilon_{xxi}}$$

Applying boundary conditions at each interface and taking $\frac{i\epsilon_{xz}}{\epsilon_{sh}} \to q$ in regions 4 and 6, gives a system of boundary condition equations $A_{mat}X = 0$, where $A_{mat}$ is

$$\begin{pmatrix}
1 & -1 & -e^{-k_m a} & 0 & 0 & 0 & 0 & 0 & 0 & 0 & 0 & 0 & 0 & 0 \\
\frac{k_{air}}{\epsilon_{air}} & \frac{k_m}{\epsilon_m} & -\frac{k_m}{\epsilon_m}e^{-k_m a} & 0 & 0 & 0 & 0 & 0 & 0 & 0 & 0 & 0 & 0 & 0 \\
0 & e^{-k_m a} & 1 & -1 & -e^{-k_{iso} b} & 0 & 0 & 0 & 0 & 0 & 0 & 0 & 0 & 0 \\
0 & \frac{k_m}{\epsilon_m}e^{-k_m a} & -\frac{k_m}{\epsilon_m} & -\frac{k_{iso}}{\epsilon_{iso}} & \frac{k_{iso}}{\epsilon_{iso}}e^{-k_{iso} b} & 0 & 0 & 0 & 0 & 0 & 0 & 0 & 0 & 0 \\
0 & 0 & 0 & e^{-k_{iso} b} & 1 & -1 & -e^{-k_{sh} l_s} & 0 & 0 & 0 & 0 & 0 & 0 & 0 \\
0 & 0 & 0 & \frac{k_{iso}}{\epsilon_{iso}}e^{-k_{iso} b} & -\frac{k_{iso}}{\epsilon_{iso}} & -\frac{(k_{sh} \pm q k_x)}{\epsilon_{sh}} & \frac{(k_{sh} \mp q k_x)}{\epsilon_{sh}}e^{-k_{sh} l_s} & 0 & 0 & 0 & 0 & 0 & 0 & 0 \\
0 & 0 & 0 & 0 & 0 & e^{-k_{sh} l_s} & 1 & -1 & -e^{-k_{sh}(d-2l_s)} & 0 & 0 & 0 & 0 & 0 \\
0 & 0 & 0 & 0 & 0 & \frac{(k_{sh} \pm q k_x)}{\epsilon_{sh}}e^{-k_{sh} l_s} & -\frac{(k_{sh} \mp q k_x)}{\epsilon_{sh}} & -\frac{k_{sh}}{\epsilon_{sh}} & \frac{k_{sh}}{\epsilon_{sh}}e^{-k_{sh}(d-2l_s)} & 0 & 0 & 0 & 0 & 0 \\
0 & 0 & 0 & 0 & 0 & 0 & 0 & e^{-k_{sh}(d-2l_s)} & 1 & -1 & -e^{-k_{sh} l_s} & 0 & 0 & 0 \\
0 & 0 & 0 & 0 & 0 & 0 & 0 & \frac{k_{sh}}{\epsilon_{sh}}e^{-k_{sh}(d-2l_s)} & -\frac{k_{sh}}{\epsilon_{sh}} & -\frac{(k_{sh} \mp q k_x)}{\epsilon_{sh}} & \frac{(k_{sh} \pm q k_x)}{\epsilon_{sh}}e^{-k_{sh} l_s} & 0 & 0 & 0 \\
0 & 0 & 0 & 0 & 0 & 0 & 0 & 0 & 0 & e^{-k_{sh} l_s} & 1 & -1 & -e^{-k_{iso} b} & 0 \\
0 & 0 & 0 & 0 & 0 & 0 & 0 & 0 & 0 & \frac{(k_{sh} \mp q k_x)}{\epsilon_{sh}}e^{-k_{sh} l_s} & -\frac{(k_{sh} \pm q k_x)}{\epsilon_{sh}} & -\frac{k_{iso}}{\epsilon_{iso}} & \frac{k_{iso}}{\epsilon_{iso}}e^{-k_{iso} b} & 0 \\
0 & 0 & 0 & 0 & 0 & 0 & 0 & 0 & 0 & 0 & 0 & e^{-k_{iso} b} & 1 & -1 \\
0 & 0 & 0 & 0 & 0 & 0 & 0 & 0 & 0 & 0 & 0 & \frac{k_{iso}}{\epsilon_{iso}}e^{-k_{iso} b} & -\frac{k_{iso}}{\epsilon_{iso}} & -\frac{k_m}{\epsilon_m}
\end{pmatrix}$$

To extract the propagation constants we again solve the system of equations that accounts for the wave equation in each heterostructure layer and enforces the boundary conditions. Note, we take $\epsilon_{xz}$ to first order in the magnetic layer again, ${\epsilon_{xz}}^2 \to 0$.

$${k_x}^2 = {k_{air}}^2 + \epsilon_{air}{k_0}^2$$
$${k_x}^2 = {k_m}^2 + \epsilon_m{k_0}^2$$
$${k_x}^2 = {k_{iso}}^2 + \epsilon_{iso}{k_0}^2$$
$${k_x}^2 = {k_{sh}}^2 + \epsilon_{sh}{k_0}^2$$
$$Det[A_{mat}] = 0$$

The spin-diffusion and thickness dependent magnetoplasmonic signal is obtained from numerically solving this system for both current orientations ($\pm i_{ac}$).

$$\left|\Delta k_{mp}\right|(d, l_s) = \left|k_x^{+i_{ac}}(d, l_s) - k_x^{-i_{ac}}(d, l_s)\right|$$
